# Supplementary material for: Spectral distortions of astrophysical blackbodies as axion probes
Source: arXiv:2305.03749 source file (2023-05-05)
Supplement: Supplementary file 1 [file appendix.tex]

\appendix 
\section{Axion-MSW}
In this section we derive the axion-Maxwell equation from scratch. The main referenec are arXiv:1903.05088v2 and https://doi.org/10.1103/PhysRevD.37.1237. Starting by writing down the Lagrangian. 
\begin{equation}
    {\cal L} \supset \frac{1}{2}\partial_\mu a \partial^{\mu} a -\frac{1}{2}m_a^2a^2 -\frac{1}{4}F_{\mu\nu}F^{\mu\nu}-\frac{1}{4}g_{a\gamma}a F_{\mu\nu}\tilde{F}^{\mu\nu}
\end{equation}
The field tensor are $F^{\mu\nu} = \partial^\mu A^\nu - \partial^\nu A^\mu$ and $\tilde{F}^{\mu\nu} = \epsilon^{\mu\nu\rho\sigma} F_{\rho\sigma}$. The equation of motion with respect to $a,A^\mu$ are
\[
\partial^{\mu} \partial_\mu a + m_a^2a +\frac{1}{4}g_{a\gamma}F_{\mu\nu}\tilde{F}^{\mu\nu}=0
\]

\[
\partial_\nu F^{\mu\nu} + g_{a\gamma} \partial_\nu a \tilde{F}^{\mu\nu} = 0
\]
[need to check to relative sign]. For historical reason we choice the gauge such that $A_0=0$. Then we can simplify the equation with respect to $a, A_i$ (I will use $A$ for $\Vec{A}$), we also separate the $\mu=0$ part and $\mu=i$ part of EoM.
\[
\partial^{\mu} \partial_\mu a + m_a^2a +g_{a\gamma}\dot{A}\cdot \nabla\times  A=0
\]
\[
\nabla \cdot \dot{A} = g_{a\gamma}\nabla a \cdot (\nabla \times A)
\]
\[
\Ddot{A}-\nabla^2A+\nabla(\nabla\cdot A) = g_{a\gamma}\dot{a}\nabla \times A-g_{a\gamma}\nabla{a} \times \dot{A} 
\]
Then we do perturbation theory. Let's say
\[
A = A_b + \delta A
\]
Under a uniform background B field. We have $\nabla \times A_b = B $ and $\dot{A}_b = 0$. From the second equation we have $\nabla \cdot \dot{A} = 0$ at the background level yield $\nabla \cdot A_b$ is constant in time and space. So the background level equations are just
\[
\Ddot{A_b}-\nabla^2A_b =0
\]
And perturbation equation
\[
\partial^{\mu} \partial_\mu a + m_a^2a +g_{a\gamma}\delta \dot{A}\cdot B=0 
\]
\[
\nabla \cdot \delta \dot{A} = g_{a\gamma}\nabla a \cdot B
\]
\[
\delta \Ddot{A}-\nabla^2\delta A + \nabla(\nabla\cdot \delta A) = g_{a\gamma}\dot{a} B
\]

The coupled equations of motion for photon and axion can be linearized and written in the following Schrodinger form
\begin{align}
    i\partial_z\begin{pmatrix}
        c_\gamma\\
        c_a
    \end{pmatrix}=\begin{pmatrix}
        \omega+\Delta_\gamma &\Delta_{a\gamma}\\
        \Delta_{a\gamma} &\omega+\Delta_a
    \end{pmatrix}\begin{pmatrix}
        c_\gamma\\
        c_a
    \end{pmatrix}
\end{align}
where
\begin{align}
    \Delta_\gamma&=-\frac{\omega_p^2}{2\omega}\\
    \Delta_a&=-\frac{m_a^2}{2\omega}\\
    \Delta_{a\gamma}&=\frac{g_{a\gamma\gamma}B}{2}
\end{align}
The only assumption that goes into deriving the above equations is that the axion/photon is relativistic, i.e. $-i\partial_j c_{\gamma,a}\approx \omega c_{\gamma,a}$.

\subsection{Small mixing regime}
Using the following ansatz
\begin{align}
    c_\gamma (z)&=\tilde{c}_\gamma (z)e^{-i\int_0^z dz' (\omega+\Delta_\gamma)}\\
    c_a (z)&=\tilde{c}_a (z)e^{-i\int_0^z dz' (\omega+\Delta_a)}
\end{align}
we can rewrite the equation for $c_a$ as
\begin{align}
    i\partial_z \tilde{c}_a=\Delta_{a\gamma}\tilde{c}_\gamma e^{-i\int_0^z dz'(\Delta_\gamma-\Delta_a)}
\end{align}
Assuming weak-mixing, $\tilde{c}_\gamma\approx 1$, the conversion probability after traversing a distance $d$ can be approximated as
\begin{align}
    P_{\gamma\rightarrow a}=\frac{1}{2}|\tilde{c}_a|^2=\frac{1}{2}\left|\int_0^{d} dz\;\Delta_{a\gamma} e^{-i\int_0^z dz'(\Delta_\gamma-\Delta_a)}\right|^2
\end{align}
where the factor of $1/2$ accounts for the fact that only one of the two linear polarizations of the photon mixes with the axion. Note that the assumption $\tilde{c}_\gamma\approx 1$ is guaranteed to be valid for our purposes because we \textit{have} observed that the spectra of all the blackbody stars are close to blackbody.

The above analysis can be trivially extend to both photon polarisation direction $\pm$. One should keep in mind when deriving the conversion probability, the crossing term should vanish over long term due to $<\tilde{c}_{\gamma-} (0)\tilde{c}_{\gamma+} (0)> = 0$. The conversion probability is

\begin{align}
    P_{\gamma\rightarrow a}=P_{\gamma+\rightarrow a}+P_{\gamma-\rightarrow a}
\end{align}
where
\begin{align}
    P_{\gamma\pm\rightarrow a}=\frac{1}{2}\left|\int_0^{d} dz\;\frac{gB_{\pm}}{2} e^{-i\int_0^z dz'(\Delta_\gamma-\Delta_a)}\right|^2
\end{align}
here $B_{\pm}$ is the projection of B field into two polarisation direction.

\subsection{Uniform medium}
In the case of a uniform medium (namely constant $B$ and $\omega_p$), the linearized photon-axion equations can be solved \textit{exactly} by projecting the photon state $\left|\gamma\right>$ onto the energy eigenstates $\left|E_{\pm}\right>$
\begin{align}
    \left|\gamma\right>&\propto \frac{2\Delta_{a\gamma}}{\Delta_a-\Delta_\gamma-\Delta_{\rm osc}}\left|E_+\right>+\left|E_-\right>\\
    E_{\pm}&=\omega+\frac{1}{2}\left(\Delta_\gamma+\Delta_a\mp \Delta_{\rm osc}\right)\\
    \Delta_{\rm osc}&=\sqrt{(\Delta_a-\Delta_\gamma)^2+4\Delta_{a\gamma}^2}
\end{align}
and evolving it
\begin{align}
    \left|\psi(z)\right>&\propto e^{-i E_- z}\left(\frac{2\Delta_{a\gamma}e^{-i(E_+-E_-)z}}{\Delta_a-\Delta_\gamma-\Delta_{\rm osc}}\left|E_+\right>+\left|E_-\right>\right)
\end{align}
The survival probability is thus given by
\begin{align}
    P_{\gamma_\parallel\rightarrow\gamma_\parallel}&= \left|\left<\gamma|\psi(L)\right>\right|^2\nonumber\\
    &\propto \left|\left(\frac{4\Delta_{a\gamma}^2}{\left(\Delta_a-\Delta_\gamma-\Delta_{\rm osc}\right)^2}\right)e^{-i \Delta_{\rm osc}L}+1\right|^2\nonumber\\
    &\propto \Delta_{\rm osc}^2-4\Delta_{a\gamma}^2\sin^2\left(\frac{\Delta_{\rm osc}L}{2}\right)
\end{align}
Normalizing the result such that $P_{\gamma_\parallel\rightarrow\gamma_\parallel}(L=0)=1$, we find
\begin{align}
    P_{\gamma_\parallel\rightarrow\gamma_\parallel}=1-\left(\frac{\Delta_{a\gamma}}{\Delta_{\rm osc}/2}\right)^2\sin^2\left(\frac{\Delta_{\rm osc}L}{2}\right)
\end{align}
and thus
\begin{align}
    P_{\gamma_{\parallel\rightarrow a}}=\left(\frac{g_{a\gamma\gamma}BL}{2}\right)^2\left(\frac{\sin(\Delta_{\rm osc} L/2)}{\Delta_{\rm osc} L/2}\right)^2
\end{align}

\subsection{Constant $B$ field, linearly varying $\omega_p^2$}
\label{appendix:linearomegapsq}
In a medium with a constant magnetic field and linearly varying plasma mass squared
\begin{align}
    \omega_p^2(z)=\omega_{p,0}^2\left(1+\frac{d-z}{L_{p}}\right)
\end{align}
the conversion probability is given by
\begin{align}
    P_{\gamma\rightarrow a}&=\left|\frac{g_{a\gamma\gamma}B}{2}\int_0^d dz\; e^{i\Phi(z)}\right|^2\\
    \Phi(z)&=\frac{1}{2\omega}\int_0^z dz'[\omega_p^2(z')-m_a^2]
\end{align}
With the benefit of hindsight, we know that the result is some combination of error function, which is defined as
\begin{align}
    \text{Erf}(z)=\frac{2}{\sqrt{\pi}}\int_0^z dt\; e^{-t^2}
\end{align}
Notice that in the error function integral the variable we are integrating over is \textit{purely quadratic} in the argument of the exponential and its integration range \textit{starts from zero}. Utilising the freedom to add a $z$-independent phase in the $P_{\gamma\rightarrow a}$ integral, we can shift the phase $\Phi(z)$ such that it is zero at the point where $\omega_p^2(z)=0$, namely
\begin{align}
    z_*=d-\left(\frac{m_a^2-\omega_{p,0}^2}{\omega_{p,0}^2}\right)L_{p}
\end{align}
As a result of this shift, we will have $\Phi(z)=-(\omega_{p,0}^2/4\omega L_p) (z-z_*)^2$, i.e. a form similar to what appears in the error function integral with $t^2=i\omega_{p,0}^2(z-z_*)^2/4\omega L_p$.

What is left is figuring out the relevant integration ranges, keeping in mind that the error function integral always starts from 0. If $z_*$ lies outside the range $[0,d]$ then $t^2$ is monotonically varying from $t^2(0)=i\omega_{p,0}^2z_*^2/4\omega L_p$ to $t^2(d)=i\omega_{p,0}^2(d-z_*)^2/4\omega L_p$ and so the $z$ integral is given by the difference of two error functions which ``start" from $t^2=0$ (the overall sign does not matter as we are taking the absolute value); If $z_*$ lies inside the range $[0,d]$ then $t^2$ goes from $t^2(0)=i\omega_{p,0}^2/4\omega L_p$ to zero before turning to $t^2(d)=i\omega_{p,0}^2(d-z_*)^2/4\omega L_p$ and so the $z$ integral is given by the sum of two error functions. Therefore the result is \textcolor{red}{[xuheng 02/26] Using the fact the Erf function is an odd function, the piecewise expression can be simplified into one.  The intergral range is not correctly given, there should be sqrt}

\begin{widetext}
\begin{align}
    P_{\gamma\rightarrow a}=\begin{cases}
    \left(\frac{g_{a\gamma\gamma}Bd}{2}\right)^2\left(\frac{\pi \omega L_p}{\omega_{p,0}^2d^2}\right)\left|\text{Erf}\left[i\frac{\omega_{p,0}^2}{4\omega L_p}(d-z_*)^2\right]-\text{Erf}\left[i\frac{\omega_{p,0}^2}{4\omega L_p}z_*^2\right]\right|, &z_*\notin [0,d] \text{ (non-resonant)}\\
    \left(\frac{g_{a\gamma\gamma}Bd}{2}\right)^2\left(\frac{\pi \omega L_p}{\omega_{p,0}^2d^2}\right)\left|\text{Erf}\left[i\frac{\omega_{p,0}^2}{4\omega L_p}(d-z_*)^2\right]+\text{Erf}\left[i\frac{\omega_{p,0}^2}{4\omega L_p}z_*^2\right]\right|, &z_*\in [0,d]\text{ (resonant)}
    \end{cases}
\end{align}
\end{widetext}

\subsection{WKB, uniform medium}
Then we do WKB approximation We assume the monochromatic plane wave are propogating in z direction with angular frequency $\omega$ so we make the ansatz
\[
a = a(z)e^{-i\omega t+i\omega z} +cc.
\]
\[
\delta A_i = -i(A_i(z)e^{-i\omega t+i\omega z} +cc.)
\]
Here $a(z), A_i(z)$ are the amplitude slow varying on z. If B field is in orthogonal to z direction, say x axis, then the second equation is zero, then we have $\partial_z A_3 = 0$. Then it is easy to see that $A_2$ still follows standard EM wave. while $A_1$ will have mixing with axion:
\begin{equation}
  \Bigg[\partial_z +   \begin{pmatrix}
0 & -g_{a\gamma}B\\
-g_{a\gamma}B & \frac{m_a^2}{\omega}
\end{pmatrix}\Bigg]
\begin{pmatrix}
A_1(z)\\
a(z)
\end{pmatrix}
\end{equation}
There is exact solution to this equation. We are particular interested the photon to axion conversion probability, defined as $P \equiv |a(L)|^2/(|a(L)|^2+|A_1(L)|^2)$, where L is the distance traveled under the B field.
\[
P = \frac{\sin^2{(gBL\sqrt{1+\frac{m_a^4}{4B^2g^2\omega^2}}})}{1+\frac{m_a^4}{4B^2g^2\omega^2}}
\]
 We are in the regime $gBL \ll 1 $, so if $\omega \gtrsim m_a^2L/2$ the conversion rate is approaching the maximum conversion $P \approx (gBL)^2$, while if $\omega \lesssim m_a^2L/2$ the conversion rate is approximately zero.

 [12/15 update]

 In the case the plasma mass is non-zero, the $m_a^2$ in the conversion probability will be replaced with $m_p^2-m_a^2$. This will reduce the conversion probability if the mass is too large. For $m_p = 4\times 10^{-12}$ eV and 100pc, this requires 130eV photon to have resonance.

 \section{Simple Magnetic Field Model and the Axion Conversion for white drawf}

The simplest magnetic field model to descibe the magnetic field of magnetized white drawf is a dipole. This is shown to decribe the magnetic field to percent level accuracy. Say the magnetic field at the pole is $B_0$, the magnetic field outside can be expressed as
\[
B = \frac{B_0R_{WD}^3}{2r^3}(3(\hat{m}\cdot \hat{r})\hat{r}-\hat{m})
\]
where $\hat{r}$ is the radial direction and $\hat{m}$ is the direction of the dipole.

To calculate the conversion rate of white drawf photon. We need to calculate the conversion rate for each trajectory that photon can reach us then sum over the surface. But in general, the magnetic field direction changes along the trajectory. So we cannot use the two component description above, instead we should do the full solution of axion propagation.

To simply the question, we will assume the typical conversion rate of a propagation direction is the conversion rate of radial trajectory original from center of MWD. This will underestimate the conversion for magnetic polar area, where the transverse B field is zero for radial trajectory. Yet, accoding to [Chrisdopher's paper] the conversion rate agree with the detailed numerical calculation up to xxx\%.

For the radial trajectory, the transvers magnetic field is always in one direction, the magnetitude is
\[
B_T = \frac{B_0R_{WD}^3}{2r^3}\sin{\theta}
\]

here $\theta$ is the altitude angle w.r.t the magnetic pole. The conversion rate is:
\[
p =\frac{(g_{a\gamma\gamma}B_0R_{WD})^2}{16}|\int_1^\infty \frac{e^{i\Delta_a r}dr}{r^3}|^2\sin^2{\vartheta}
\]
where $\vartheta$ is the incline angle of the observatory and $\Delta_a = \frac{m_a^2R_{WD}}{2E}$. The numerical result of the energy dependent factor $F(\delta_a) \equiv |\int_1^\infty \frac{e^{i\delta_a r}dr}{r^3}|^2$ is shown in the plot \ref{fig1}.
\begin{figure}
\includegraphics[width=0.95\columnwidth]{Overleaf/Plot/output.png}
\caption{\label{fig1}}
\end{figure}

This can be writtrn in closed form
[03/15 xuheng] by integrate-by-parts twice.

\textcolor{red}{Magnetic White Drawf Conversion Rate}
\[
p =\frac{(g_{a\gamma\gamma}B_0R_{WD})^2\sin^2{\vartheta}}{64}|1 + i\Delta_a -\Delta_a^2e^{-i\Delta_a}\int_{\Delta_a }^\infty \frac{e^{ir}dr}{r}|^2
\]
There the integral can be rewrite into real arguement function by Euler equation
\[
\int_{\Delta_a }^\infty \frac{e^{ir}dr}{r} = -ci(\Delta_a)-isi(\Delta_a)
\]
with defination of this special function (available in mma and python)
\[
ci(x) = -\int_x^\infty\frac{\cos(x)}{x}
\]
\[
si(x) = -\int_x^\infty\frac{\sin(x)}{x}
\]

Cross checked the result, this is correct expression. The conversion is a monotomic funtion of energy, there is no fluctuation. 

\begin{figure}
\includegraphics[width=0.95\columnwidth]{Overleaf/Plot/output3.png}
\caption{\label{fig1}}Axion photon conversion in white drawf atmosphere, R = 6000km, B = $10^7$G, $g_{a\gamma} = 10^{-11}\rm{GeV}^{-1}$
\end{figure}

 \section{QED Birefringence}
 
 Check arXiv:1903.05088v2 for more details. It is well known the Maxwell give correct prediction under weak field compared with Schwinger limit. If the background field is strong enough, the loop order correction should be included
 \begin{equation}
    {\cal L} \supset \frac{\alpha^2}{90m_e^4}[(F_{\mu\nu}F^{\mu\nu})^2+\frac{7}{4}(F_{\mu\nu}\tilde{F}^{\mu\nu})^2]
\end{equation}

For our interests, this modifed the EoM of photon and appear to be like a effective (negative) mass term, for 2-component cases, the effective mass looks like
\[
m_{QED}^2(r) = -7 \omega^2\frac{\alpha}{45\pi} (\frac{B_T(r)}{B_{crit}})^2
\]

$B_{crit} = 4.41 \times 10^{13} G$ This is only important at strong magnetic field. But have a great potential reach (we are no longer in need of ma to get energy dependence, so ma can go to zero).

\[
\Delta_{QED} = m_{QED}^2/2\omega \approx 10^{-15}(\frac{B}{100 MG})^2\frac{\omega}{1eV} eV 
\]
\[
\Delta_B = \frac{1}{2}g_{a\gamma\gamma}B = 10^{-15}\frac{g_{a\gamma\gamma}}{10^{-12}GeV^{-1}}\frac{B}{100MG}eV
\]
The conversion rate is
\[
p =\frac{(g_{a\gamma\gamma}B_0R_{WD})^2}{16}|\int_1^\infty \frac{e^{\int i\Delta_{QED} dr}dr}{r^3}|^2\sin^2{\vartheta}
\]
where
\[
\int \Delta_{QED} dr = \frac{7}{1800\pi}\alpha \omega R_{wd} (\frac{B_0}{B_{crit}})^2 (1-(R_{wd}/r)^5)
\]
This remains small even for 1000MG

\section{WD conversion: non-radial trajectories}
\subsection{Xuheng}
 Here we analysis the conversion rate from magnetic field around WD detailly. First we need to specify the geometry. Notice that there are degree of freedom of choosing coordinates and polarisation direction in the telescope. Without loss of generisity, we set WD at the original point, the magnetic dipole is in z direction $\hat{m} = e_z$, the observer sits in the $xoz$ plane with a incline angle $\Theta$. This angle is fixed for each WD, the reader should distinguish this from $\theta$. The trajectory direction and photon polarisation direction is defined as
 \[
 e_n = \sin \Theta e_x+ \cos \Theta e_z,
 \]
 \[
 e_+ = \cos \Theta e_x - \sin \Theta e_z
 \]
 \[
 e_- = e_y,
 \]
 Then the trajectory of photon is defined as
 \[
 r = l*e_n+r_0
 \]
 \[
 \hat{r} = \frac{(\sin \Theta l+x_0,y_0,\cos \Theta l+z_0)}{\sqrt{(\sin \Theta l+x_0)^2+y_0^2+(\cos \Theta l+z_0)^2}}
 \]

 where $l$ runs from zero to infinity and $r_0$ is the original point on the WD. If the $r_0$  is also on the $xoz$ plane, the $e_-$ component should vanish due to symmetry reason. Since WD radiation is close to a blackbody, the photon we observed is uniformly distributed from the circle projected from hemisphere facing us.

 The two component of magnetic field is

 \[
 B_+ = B*e_+ = \frac{B_0R_{WD}^3*(3*(\cos \Theta l +z_0)*(\cos \Theta x_0-\sin \Theta z_0)+\sin\Theta*r^2)}{2r^5}
 \]
 \[
B_- = B*e_- = \frac{3B_0R_{WD}^3*y_0*(\cos \Theta l +z_0)}{2r^5}
 \]

 A quick check is to set $x_0 = R\sin\Theta, z_0 = R\cos\Theta, y_0 = 0$, then this go back to radial direction case.

 To get the averaged result, we need to integrate over the sphere. It is useful to use projected circular coordinate. The measure is $dA = r'd\theta'dr$ here $r', \theta'$ is on a $\Theta$ angle tilted plane facing $e_n$ direction. The corresponding initial point in the sphere is
 \[
 \frac{r_0}{R} = \sqrt{1-r'^2}e_n + (r'\cos \theta'\cos \Theta,r'\sin \theta',-r'\cos \theta'\sin \Theta)
 \]

 \[
 \frac{r_0}{R} = (\sqrt{1-r'^2}\sin \Theta +r'\cos\theta'\cos \Theta,r'\sin\theta',\sqrt{1-r'^2}\cos \Theta-r'\cos\theta'\sin \Theta)
 \]

 \begin{figure}
\includegraphics[width=0.95\columnwidth]{Overleaf/Plot/conversion_incline.png}
\caption{} conversion rate vs incline angle (E is large). The analytical form doesn't work because we underestimate the transverse direction magnetic field
\end{figure}

\begin{figure}
\includegraphics[width=0.95\columnwidth]{Overleaf/Plot/numerical_compare.png}
\caption{} The conversion rate vs energy. The inlcine angle is set to $\Theta = \pi/2$ The analytical form agree with the numerical form.
\end{figure}

\clearpage
\newpage

\subsection{Erwin}
To take advantage of the azimuthal symmetry of the dipole magnetic field, we work in the spherical coordinates $(r,\theta,\phi)$ with $\hat{z}=\hat{m}$. The white dwarf magnetic field reads
\begin{align}
    \vec{B}=\frac{B_0R^3}{2r^3}\left[3(\hat{z}.\hat{r})\hat{r}-\hat{z}\right]
\end{align}
The position vector $\vec{r}$ of a photon emitted from $\hat{r}=R\hat{r_{\rm em}}$ and observed at infinity in the direction $\hat{r}_{\rm obs}$ can be parameterized as
\begin{align}
    \vec{r}=R\hat{r}_{\rm em}+\chi R\hat{n}_{\rm obs}
\end{align}
where $\chi$ goes from $0$ to $\infty$. The magnitude of $\vec{r}$ is given by
\begin{align}
    \tilde{r}(\chi)\equiv\frac{|\vec{r}|}{R}=\sqrt{1+\chi^2+2\chi\hat{r}_{\rm em}.\hat{n}_{\rm obs}}
\end{align}
where 
\begin{align}
    \hat{r}_{\rm em}.\hat{n}_{\rm obs}=\sin\theta_{\rm em}\sin\theta_{\rm obs}\cos\phi_{\rm em}+\cos\theta_{\rm em}\cos\theta_{\rm obs}
\end{align}
and we have aligned the spherical coordinates such that $\phi_{\rm obs}=0$. The magnetic field parallel to the photon trajectory is
\begin{widetext}
\begin{align}
    B_L=\frac{B_0R^3}{2r^3}\left[3(\hat{z}.\hat{r})(\hat{r}.\hat{n}_{\rm obs})-\hat{z}.\hat{n}_{\rm obs}\right]=\frac{B_0}{2\tilde{r}^3}\left[3\left(\frac{\cos\theta_{\rm em}+\chi\cos\theta_{\rm obs}}{\tilde{r}}\right)\left(\frac{\hat{r}_{\rm em}.\hat{n}_{\rm obs}+\chi}{\tilde{r}}\right)-\cos\theta_{\rm obs}\right]
\end{align}
\end{widetext}
and the components orthogonal to the trajectory are
\begin{widetext}
    \begin{align}
    B_{T,1}&=\frac{B_0}{2\tilde{r}^3}\left[3\left(\frac{\cos\theta_{\rm em}+\chi\cos\theta_{\rm obs}}{\tilde{r}}\right)\frac{1+\chi\hat{r}_{\rm em}.\hat{n}_{\rm obs}}{\tilde{r}}\sin \theta_{\rm em}\sin \phi_{\rm em}\right] \\
    B_{T,2}&=\sqrt{B_{T}^2-B_{T,1}^2}
\end{align}
\end{widetext}
with
\begin{align}
    B_T&=\sqrt{B^2-B_L^2}\\
    B&=\sqrt{\vec{B}.\vec{B}}=\frac{B_0}{2\tilde{r}^3}\sqrt{1+3\left(\frac{\cos\theta_{\rm em}+\chi\cos\theta_{\rm obs}}{\tilde{r}}\right)^2}
\end{align}

Now that everything is parameterised in terms of $\chi$, we can do the probability integral
\begin{align}
    P_{\gamma\rightarrow a}=&\frac{1}{2}\left|\frac{g_{a\gamma\gamma}R}{2}\int_0^\infty d\chi\;B_{T,1} e^{i\delta_a \chi}\right|^2\\
    &+\frac{1}{2}\left|\frac{g_{a\gamma\gamma}R}{2}\int_0^\infty d\chi\;B_{T,2} e^{i\delta_a \chi}\right|^2
\end{align}
The ($\theta_{\rm em},\phi_{\rm em}$)-averaged probability can be found as
\begin{widetext}   
\begin{align}
    \bar{P}_{\gamma\rightarrow a}(\theta_{\rm obs})&=\frac{\int_0^{\pi/2+\theta_{\rm obs}}\int_0^{\Phi(\theta_{\rm em},\theta_{\rm obs})} d\phi\, (R|\sin\theta_{\rm em}|)(Rd\theta_{\rm em})(\hat{r}_{\rm em}.\hat{n}_{\rm obs})  P_{\gamma\rightarrow a}(\theta_{\rm em},\phi_{\rm em},\theta_{\rm obs})}{\pi R^2}\nonumber\\  
    &=\frac{1}{\pi}\int_0^{\pi/2+\theta_{\rm obs}} d\theta_{\rm em}\,|\sin\theta_{\rm em}|\int_0^{\Phi(\theta_{\rm em},\theta_{\rm obs})} d\phi\,(\hat{r}_{\rm em}.\hat{n}_{\rm obs}) P_{\gamma\rightarrow a}(\theta_{\rm em},\phi_{\rm em},\theta_{\rm obs})
\end{align}
\end{widetext}
where 
\begin{align}
    \Phi(\theta_{\rm em},\theta_{\rm obs})=2\left\{\frac{\pi}{2}+\text{min}\left[1,\sin^{-1}\left(\cot{\theta_{\rm em}}\cot\theta_{\rm obs}\right)\right]\right\}
\end{align}
is the $\phi$ excursion for a given $\theta_{\rm em}$.
